# Supplementary material for: FoPro-KD: Fourier Prompted Effective Knowledge Distillation for Long-Tailed Medical Image Recognition
Source: arXiv:2305.17421 source file (2023-12-12)
Supplement: Supplementary file 1 [file tmi-7-Appendix.tex]

\section{Appendix}
\input{tmi-5.4-Free Lunch Models}
\input{tmi-5.6-Weight Initialization Ablation}
